# Supplementary material for: Refining Semantic Segmentation with Superpixel by Transparent Initialization and Sparse Encoder
Source: arXiv:2010.04363 source file (2020-11-24)

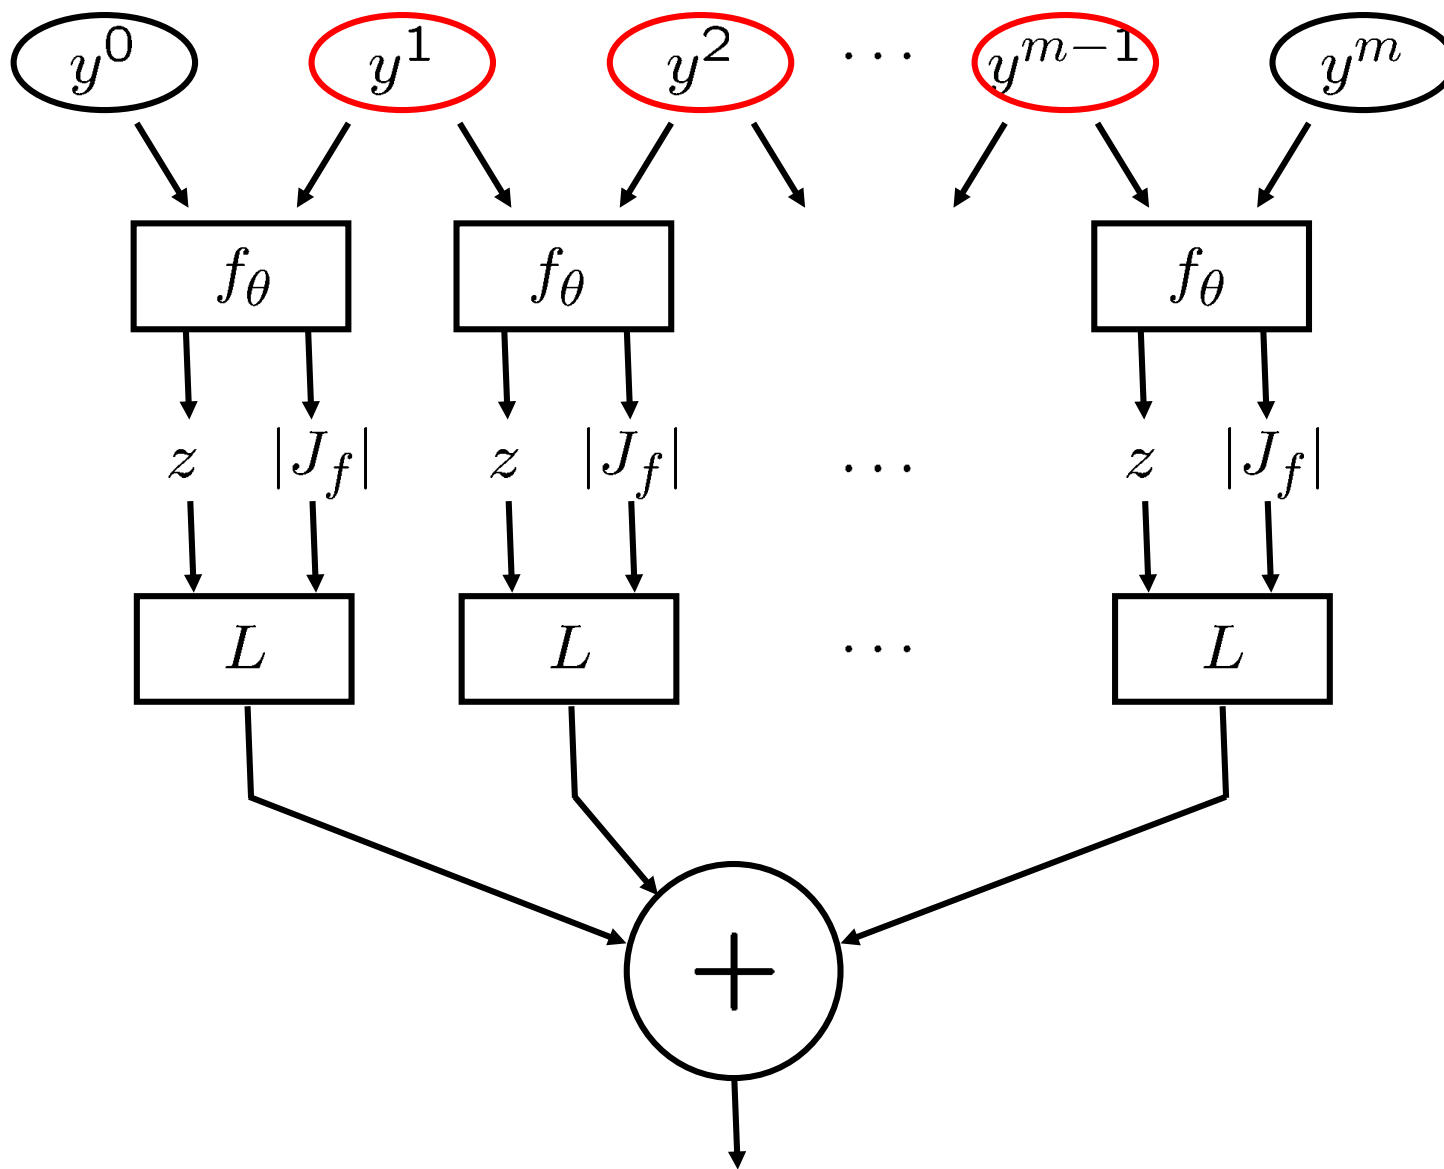

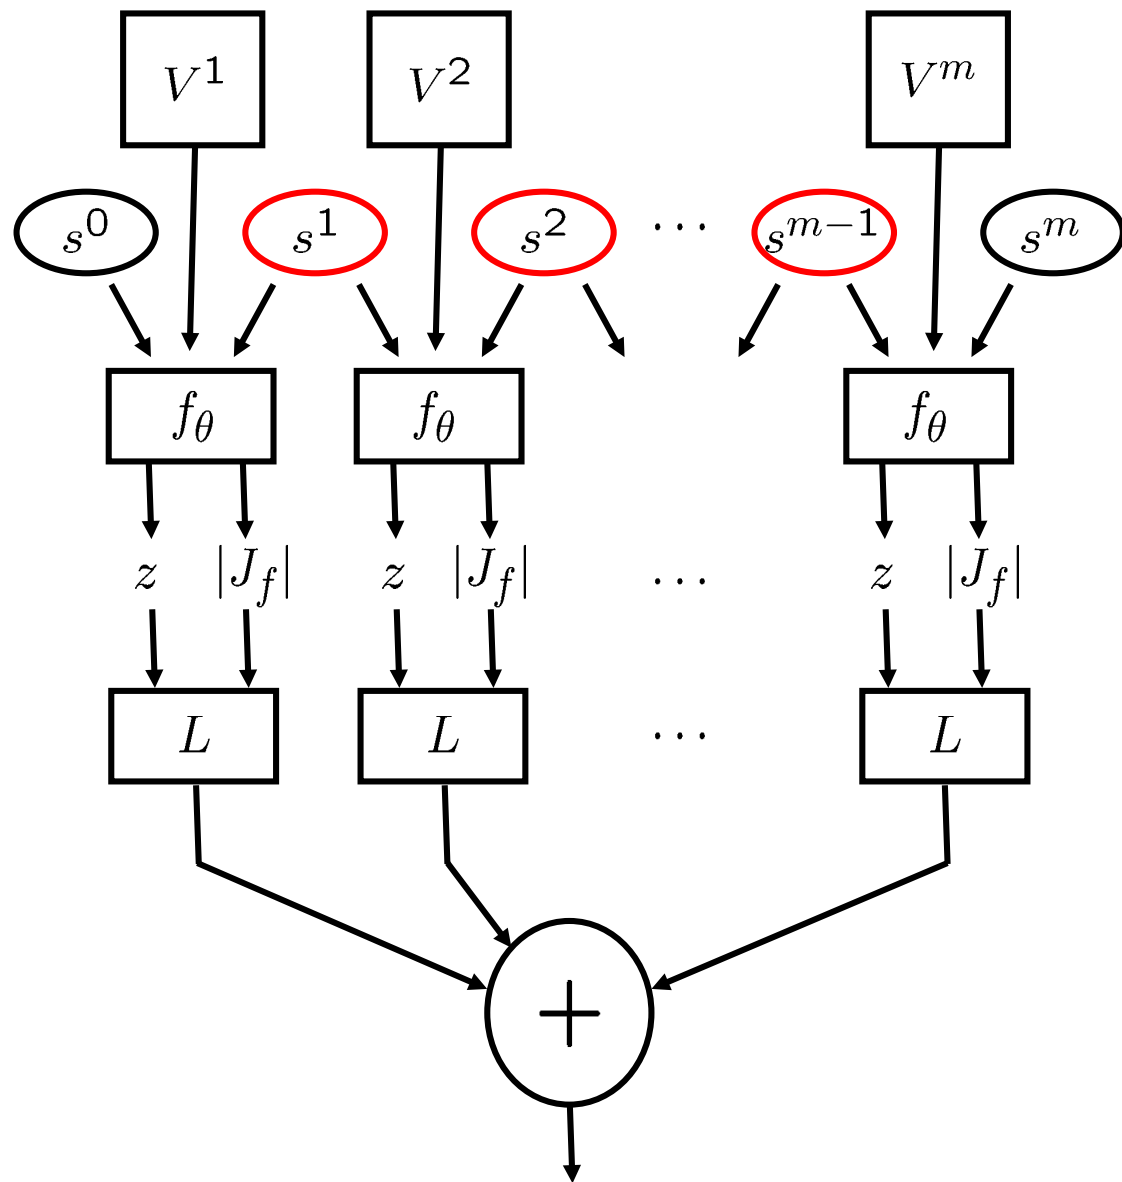

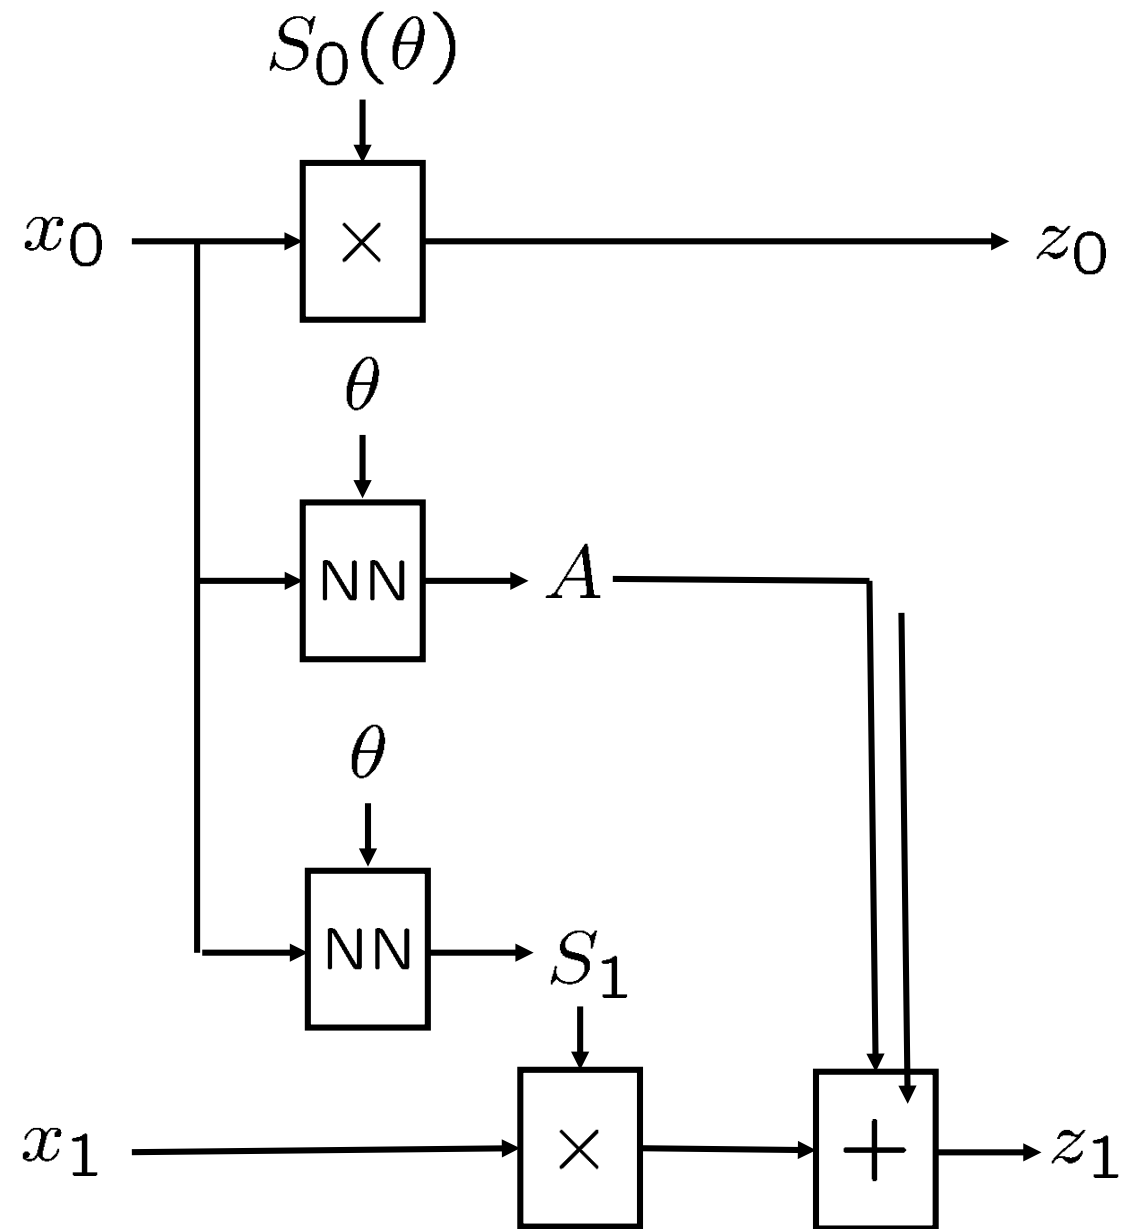

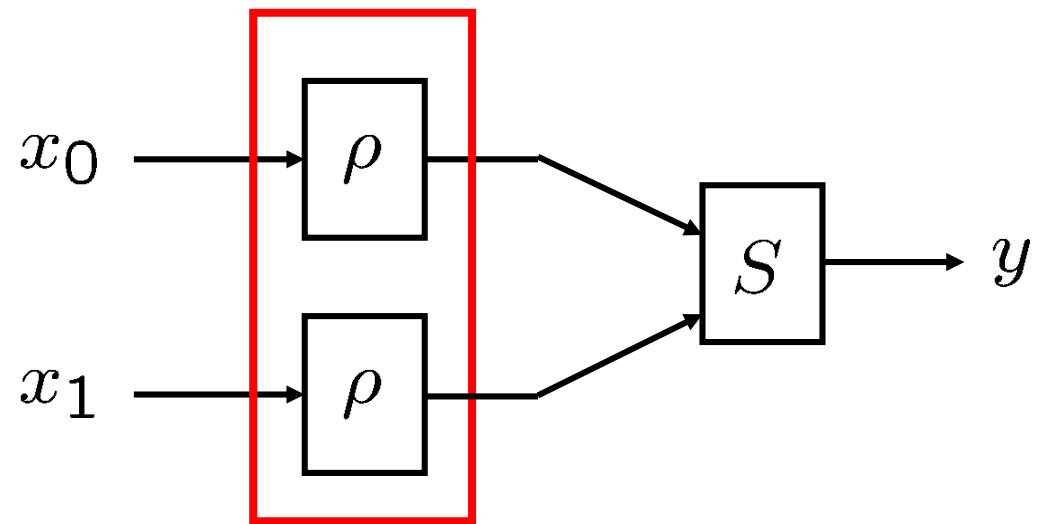

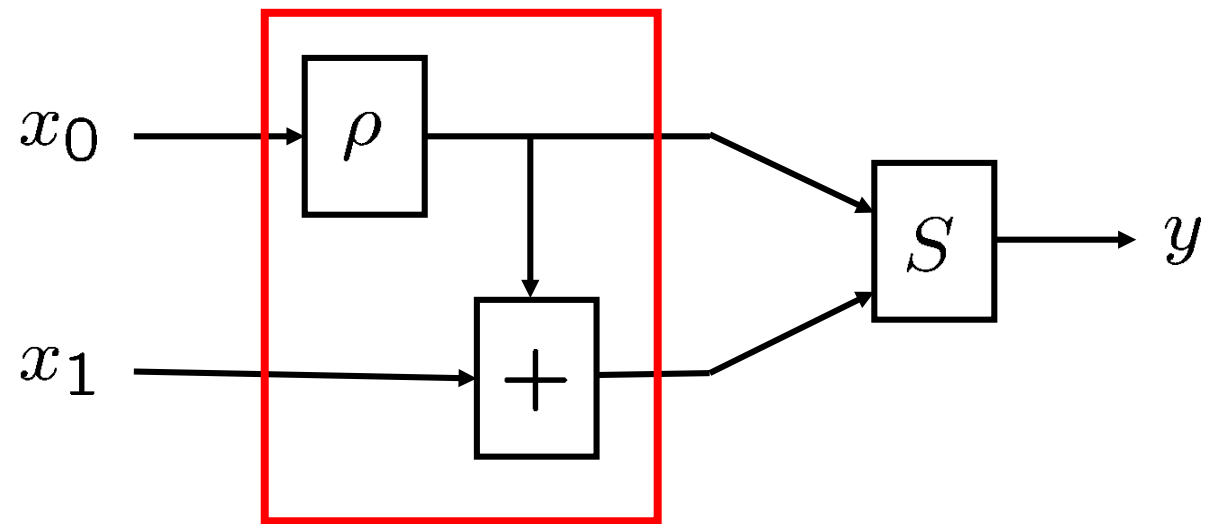

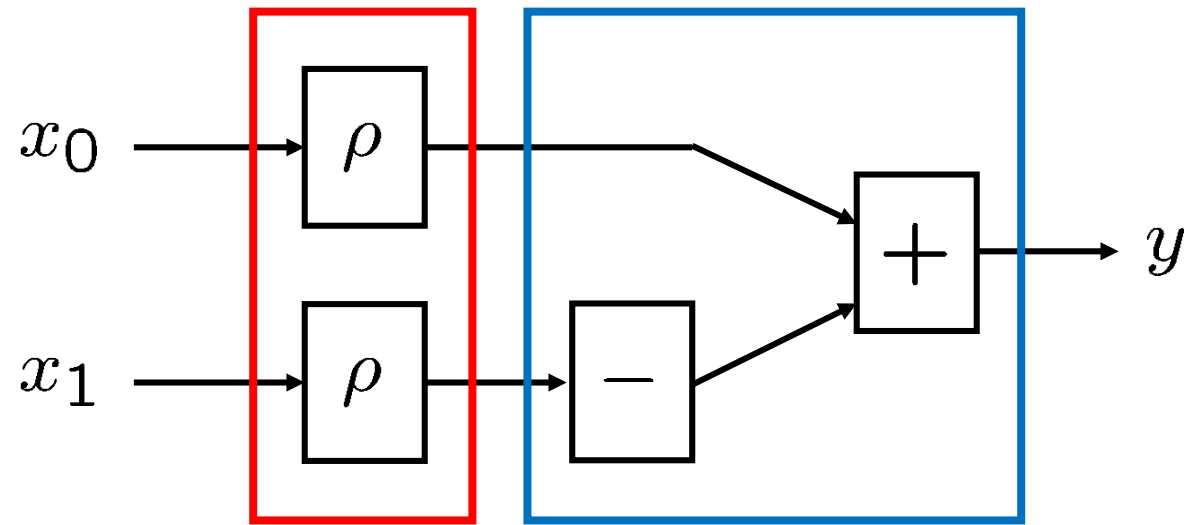

Supplement: Supplementary file 1 [file Figures.pdf]
